# Supplementary material for: LoopDraw: a Loop-Based Autoregressive Model for Shape Synthesis and Editing
Source: arXiv:2212.04981 source file (2024-05-29)
Supplement: Supplementary file 1 [file 99_supp-2024.tex]

\section{Network Architecture}
For the vase dataset, we use a batch size of 4, with 4 transformer layers (single-head), a layer embedding size of 512, a fully-connected layer size of 512, and latent $\mathbf z$ prediction/$\mathbf d$ prediction MLPs with a single hidden layer of size 128. 
For the ShapeNet sofa dataset, we use a batch size of 16, with 8 transformer layers (each with 8 heads), a layer embedding size of 512, a fully-connected layer size of 768, and latent $\mathbf z$ prediction/$\mathbf d$ prediction MLPs with two hidden layers of size 128. 
Both models employ a latent code size of $N_z = 64$. \rhc{TODO: do you have reason why they are different?}

\section{Comparisons}
\rhc{TODO: move this section to the supp}
\label{sec:metrics}
\rhc{TODO: very sparse and lightweight representation}
\paragraph{Quantitative evaluation}
As far as we are aware, \ourmethod{} is the first technique to use an autoregressive loop primitive for shape synthesis and editing. Since existing techniques take as input alternative representations (such as point clouds, voxels, or tetrahedra), our evaluations inevitably compare across VAEs with different input types. Thus, we compare against various other representations used for generating 3D shapes: Occupancy Networks \cite{mescheder2019occupancy}, which represents surfaces with occupancy fields; ShapeGAN's provided VAE variant \cite{kleineberg2020shapegan} (for encoding \& reconstruction capability), which uses signed distance fields as its decoder shape representation; and TetGAN \cite{gao2022tetgan}, which is a volumetric representation, in \cref{tab:fid-metrics}.
The reconstruction tests evaluate the average Chamfer distance between ground truth shapes and the reconstructed shapes, sampled as point clouds.
The FID tests evaluate the FID-based distance between a test set and a batch of 250 random samples, utilizing deep features from a pre-trained PointNet \cite{qi2017pointnet} classification network.

% We evaluate the metrics for our method on two different surface measures. The first measure compares the fit of our predicted loops compared against loops from the reference set. The second measure reconstructs a surface using Poisson reconstruction and then compares the surface against the underlying surfaces from the reference set. % not doing this anymore
Our results show that, in addition to the interpretability and editability of loops, LoopDraw's reconstruction and FID performance are on par with the other representations tested. \rh{We stress that our method is designed to enable \textit{conditional} editing and manipulation capabilities, rather than more traditional unconditional synthesis.}

\paragraph{Qualitative comparisons}
\begin{figure*}
    \centering
    \includegraphics[scale=1.2]{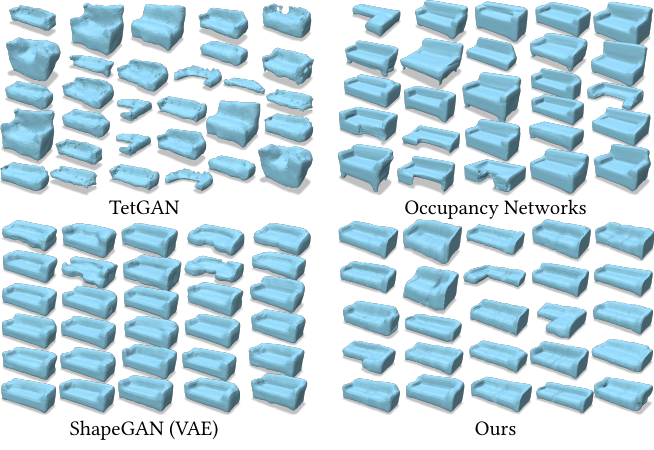}
    % \begin{tikzpicture}[scale=0.7]
    % \node[anchor=base,inner sep=0] at (3.5,0){ShapeGAN (VAE)};
    % \node[anchor=south west,inner sep=0] at (0,0.5) {\includegraphics[width=0.3\linewidth]{figures/comparisons/sofa/shapeganvae-stitch.png}};
    % \node[anchor=base,inner sep=0] at (12,0){Ours};
    % \node[anchor=south west,inner sep=0] at (8.2, 0.5) {\includegraphics[width=0.3\linewidth]{figures/comparisons/sofa/ours-stitch.png}};
    % \node[anchor=base,inner sep=0] at (3.5,5.35){TetGAN};
    % \node[anchor=south west,inner sep=0] at (0, 5.8) {\includegraphics[width=0.3\linewidth]{figures/comparisons/sofa/tetgan-stitch.png}};
    % \node[anchor=base,inner sep=0] at (12,5.35){Occupancy Networks};
    % \node[anchor=south west,inner sep=0] at (8.2, 5.8) {\includegraphics[width=0.3\linewidth]{figures/comparisons/sofa/occnet-stitch.png}};
    
    % \end{tikzpicture}
    \caption{Visual results for the Sofas category from our quantitative comparison in \cref{tab:fid-metrics}. We compare our random samples of sofas with samples from the other three methods trained on the same dataset.}
    \label{fig:visual-comparison}
\end{figure*}
\begin{figure*}
\centering
    \includegraphics[scale=1.2]{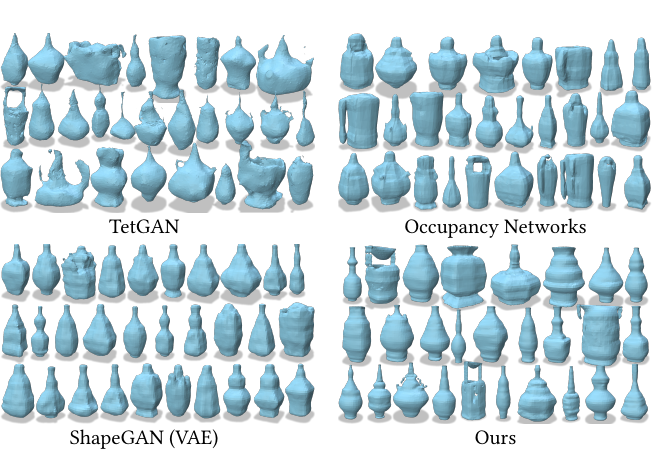}
    % \begin{tikzpicture}[scale=0.7]
    % \node[anchor=base,inner sep=0] at (3.5,0){ShapeGAN (VAE)};
    % \node[anchor=south west,inner sep=0] at (0,0.5) {\includegraphics[width=0.3\linewidth]{figures/comparisons/vases/shapeganvae-stitch.png}};
    % \node[anchor=base,inner sep=0] at (12,0){Ours};
    % \node[anchor=south west,inner sep=0] at (8.2, 0.5) {\includegraphics[width=0.3\linewidth]{figures/comparisons/vases/ours-stitch.png}};
    % \node[anchor=base,inner sep=0] at (3.5,5.1){TetGAN};
    % \node[anchor=south west,inner sep=0] at (0, 5.6) {\includegraphics[width=0.3\linewidth]{figures/comparisons/vases/tetgan-stitch.png}};
    % \node[anchor=base,inner sep=0] at (12,5.1){Occupancy Networks};
    % \node[anchor=south west,inner sep=0] at (8.2, 5.6) {\includegraphics[width=0.3\linewidth]{figures/comparisons/vases/occnet-stitch.png}};
    
    % \end{tikzpicture}
    \caption{Visual results for the Vases category from our quantitative comparison in \cref{tab:fid-metrics}. We compare our random samples of vases with samples from the other three methods trained on the same dataset.}
    \label{fig:visual-comparison-vases}
\end{figure*}

We gather random samples from each method trained on the COSEG vase and ShapeNet sofa datasets (\cref{fig:visual-comparison,fig:visual-comparison-vases}). We note that \ourmethod{}'s visual quality and structural variety are competitive with these volumetric and implicit surface methods. In particular, both ours and Occupancy Networks strike a similar balance between visual quality and geometric diversity, despite differing in their FID scores.
Our results also show features (e.g., indents resembling separate cushions on a sofa) not well-captured by the other methods.

\begin{table}[]
    {\small
    \centering
    \begin{tabular}{cccc}
    \toprule
    Category & Method & Reconstruction $\downarrow$ & FID $\downarrow$  \\
    \midrule
    \multirow{4}{*}{Vases} & Occupancy Net. & 0.0187 & 7.42  \\ 
    {} & ShapeGAN (VAE)& 0.0048 & 20.51 \\
    {} & TetGAN & 0.0055 & 2.57  \\
    {} & \textit{Ours} & 0.0184 & 4.43  \\
    \midrule
    \multirow{4}{*}{Sofas} & Occupancy Net. & 0.0118 & 1.54  \\
    {} & ShapeGAN (VAE)& 0.0018 & 8.30  \\
    {} & TetGAN & 0.0024 & 3.35  \\
    {} & \textit{Ours} & 0.0109 & 8.77  \\
    \bottomrule
    \end{tabular}
    }
    \caption{FID and reconstruction evaluation for the three shape categories, with comparisons to other methods.\rhc{TODO: move this to the supp and replace with edit figs} \nmc{TODO UPDATE WITH NEW NUMBERS (from no-prevent-thin-loops metrics)}}
    \label{tab:fid-metrics}
\end{table}
